# Supplementary material for: The role of interfacial adhesion on minimum wear particle size and roughness evolution
Source: arXiv:2003.10192 source file (2020-03-23)

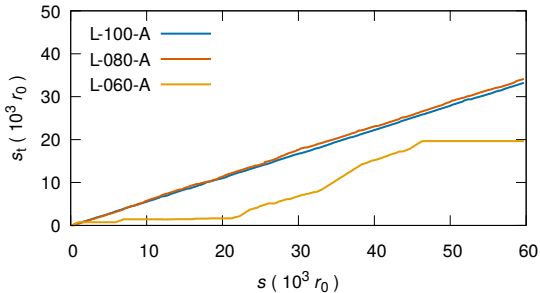

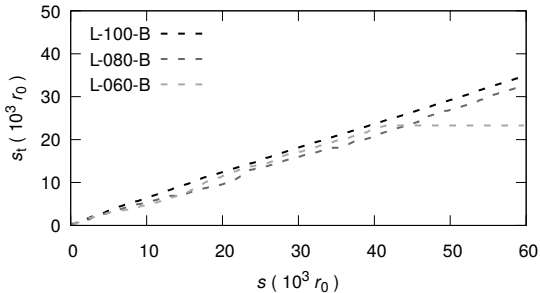

Supplement: Supplementary file 1 [file travel_supp_1.pdf]
